# Supplementary material for: Stellar population astrophysics (SPA) with the TNG: Measurement of the He I 10830{\AA} line in the open cluster Stock 2
Source: arXiv:2404.09975 source file (2024-04-15)
Supplement: Supplementary file 1 [file rev1_cover_letter.tex]

\documentclass{article}

\usepackage{xcolor}
  \definecolor{sx-yellow}{RGB}{249,245,233}
  \definecolor{sx-orange}{RGB}{224,215,188}
\usepackage[most]{tcolorbox}

\newcommand{\xtnote}[1]{\textit{\textcolor{orange}{[xiaoting:#1]}}}
\newcommand{\xt}[1]{\textcolor{orange}{#1}}
\newcommand{\mjnote}[1]{\textit{\textcolor{magenta}{[mingjie:#1]}}}
\newcommand{\mj}[1]{\textcolor{magenta}{#1}}

\makeatletter
\renewenvironment{quote}{%
  \vskip 10\p@
  \parindent\z@
  \tcolorbox[
    breakable, sharp corners,
    boxrule=\z@, boxsep=\z@,
    left=\z@, right=\z@,
    top=\z@, bottom=\z@,
    colback=sx-yellow
  ]
  {\color{sx-orange}\d@ublerule}
  \vskip 5\p@
  \list{}{\rightmargin\leftmargin}%
  \item\relax
}{%
  \endlist
  {\color{sx-orange}\d@ublerule}
  \endtcolorbox
  \vskip 5\p@
}
\def\d@ublerule{\hrule\@width\hsize\kern 1.5\p@\hrule\@width\hsize}
\makeatother


\begin{document} 

\section{Cover letter to the editor}

Thank you for managing the manuscript.
We have revised the manuscript, taking into consideration the referee's comments. 
The figures and tables have been reorganized to adhere to the A\&A guidelines, and they are now presented in the correct numerical order within the body of the text.
All the changes in the manuscript are indicated in the reply to the referees.
The clean and latexdiff version (in referee and printer format) of the manuscript are attached.  

\end{document}
