# Supplementary material for: Stellar population astrophysics (SPA) with the TNG: Measurement of the He I 10830{\AA} line in the open cluster Stock 2
Source: arXiv:2404.09975 source file (2024-04-15)
Supplement: Supplementary file 2 [file rev1_reply.tex]

\documentclass{article}

\usepackage{xcolor}
  \definecolor{sx-yellow}{RGB}{249,245,233}
  \definecolor{sx-orange}{RGB}{224,215,188}
\usepackage[most]{tcolorbox}

\newcommand{\xtnote}[1]{\textit{\textcolor{orange}{[xiaoting:#1]}}}
\newcommand{\xt}[1]{\textcolor{orange}{#1}}
\newcommand{\mjnote}[1]{\textit{\textcolor{magenta}{[mingjie:#1]}}}
\newcommand{\mj}[1]{\textcolor{magenta}{#1}}

\makeatletter
\renewenvironment{quote}{%
  \vskip 10\p@
  \parindent\z@
  \tcolorbox[
    breakable, sharp corners,
    boxrule=\z@, boxsep=\z@,
    left=\z@, right=\z@,
    top=\z@, bottom=\z@,
    colback=sx-yellow
  ]
  {\color{sx-orange}\d@ublerule}
  \vskip 5\p@
  \list{}{\rightmargin\leftmargin}%
  \item\relax
}{%
  \endlist
  {\color{sx-orange}\d@ublerule}
  \endtcolorbox
  \vskip 5\p@
}
\def\d@ublerule{\hrule\@width\hsize\kern 1.5\p@\hrule\@width\hsize}
\makeatother


\begin{document} 

\section{Reply to the referee}

We would like to thank the referee for all useful comments on the manuscript. 
Below is our response to the issues raised in the review.

\begin{quote}
    - Q1: Fig 3 contains an unidentified absorption feature in the observed spectrum at 10831.5. What is that feature? It should be identified.
\end{quote}

Reply: 
We note that this weak feature can only be seen in the star g1 in Fig. 3.
There is no telluric line in this wavelength, nor relatively strong atomic lines, thus it may happen to be a feature caused by photon noise for star g1. 
Since The fitting of profiles are not affected by any eventual feature close to this wavelength, it is not relevant to the present work. However, we plan to identify it in a future work based on a larger dataset.

\begin{quote}
    - Q2.1: Fig 6 and the extraction of the secondary helium line appears much less certain than is claimed in the text. The secondary line is very obvious in cool dwarf stars... see the many CARMENES spectra (for instance, Fuhrmeister et al, 2019, A\&A, 632, A24) where the equivalent width seems to vary between 12 and 17\% of the main feature, and has FWHM comparable to the main feature. Table 4 in this manuscript shows that the secondary components have an equivalent width of 5-11\%, and the FWHM are less by factors of 1.7 to 2 as compared to the main transition. This is interesting, yet puzzling, for it raises concerns about the reality of the secondary component. Can these discrepancies be explained?
\end{quote}

Reply: 
We agree with the referee that for these stars the secondary HeI line component is more elusive than for other stars. Indeed, we could detect it only for the three giants with the strongest HeI line, as stated in the manuscript, and we reported only indicative parameters for the secondary component, as can be inferred from the large errorbars of EW and FWHM.
Moreover, the main targets of Fuhrmeister et al. (2019) are M-type dwarfs, whose He10830 may have different behaviours compared to the FGK-type stars with different temperatures. 
The spectra shown in Takeda \& Takada-Hidai (2011, PASJ, 63, 547) tend to have similar secondary-to-main EW ratios with our work. 
Such discrepancy of the secondary He component in different kinds of stars is interesting and puzzling.
However, in order to figure out the physics behind the discrepancy requires detailed modelling of the stellar chromosphere with high precision, which is currently not available in the community and is beyond the scope of this work.

\begin{quote}
    - Q2.2: Fig 6 also demonstrates that the red wing of the main component is severely blended with the telluric line, and in several cases (and especially g2, g5, g10) the fitted main feature may not be reliable. This result would be greatly improved for the reader to understand and increase confidence in the fit, if the plots extended to at least 10834 A, so that the continuum placement could be seen. The placement of the continuum will affect the fitting of the main component, the presence of a secondary component, and also influence the presence of asymmetry (or not). Many other authors, whose data are shown in Fig. 10 have not identified a secondary component to the line in luminous stars, but interpreted the asymmetric profile as an indication of absorption from the metastable level by a stellar wind. It is interesting that targets g2 and g10 appear to have weaker “blue” Ca II K peaks than the red peak – perhaps indicative of a wind in these objects.
\end{quote}

Reply: 
Concerning the fit range of the wavelength, we aim to avoid extending the fit to 10844A because there is another telluric line at 10833.8A. Extending the plots to 10834A helps little to identify the continuum of the observed spectra. 

As the referee pointed out, some of the previous works interpreted the asymmetric line profile as stellar wind. We note that the resolutions of most of these works are around 25000, lower than that of our spectra. Further, they are more focused on metal-poor stars, which tend to have weaker Helium feature. Since the three secondary features are located in the wavelength of the weakest transition, we would like to express this as the second component.

Concerning on the Ca II K feature, in a following paper of our He10830 series, we will apply the method that introduced in this paper to red clump stars in different open clusters. With the larger sample of red clump stars in different stellar populations with different ages and stellar masses, we will reveal an even better relation between the He10830 line profile and Ca II HK lines.

\begin{quote}
    - Q3: Two X-ray satellites, CHANDRA and eRosita have released large all sky catalogs with on-line search engines. It would be interesting (and trivial to do) to check if the Stock 2 targets are included. Finding (or not) a relationship with X-ray flux might explain the 3 stars with strong helium absorption.
\end{quote}

Reply: 
We do have checked the Chandra source catalog but no X-ray measurement is available in the Stock-2 area. For other X-ray catalogues including eRosita, their angular resolution is usually large, at the order of 10", thus it would be hard to identify whether the X-ray radiation is indeed from our target star or other stars nearby. 

\begin{quote}
    - C1: Introduction, par 1...'almost all ..clusters..have stars ...forming in different epochs'... It is not as simple as that. The jury is still out. Reference: Bastian and Lardo, 2018, ARAA, 56, 83
\end{quote}

Reply: 
We put also the possible doubts and reference on the Globular Cluster formation.


\begin{quote}
    C2: Introduction, par 3: 
    
    A. the ‘ground state’ of an atom is the 0 energy level (the lowest) of the atom, and the 3S is the lowest level of the triplet sequence, but not the ground state of neutral helium.
    
    B. The text suggests that EUV photoionization becomes important for G2 and earlier. This appears to contradict the early work (and others) of Zarro \& Zirin (1986) who demonstrated the strong correlation of He line strength with X-rays in dwarf stars of F7 and later. 
    
    C. By “over-ionization” isn’t photo-ionization meant here?
    
    D. Define GIARPS... this is the first mention of that abbreviation, and so needs to be defined

\end{quote}

Reply: 
Thank you for pointing out these points. We modified the text according to the comments.

\begin{quote}
    - C3: Introduction, par -2: Reddy and Lambert derived the [Fe/H] abundance not 'metallicity.' Were the LAMOST abundances [Fe/H] also?
\end{quote}

Reply: 
The values reported in these two papers are all [Fe/H]. We have corrected these in the manuscript.

\begin{quote}
    - C4: Table 1 should include parameters of the stars, the V mag and colors, or the Gaia values.

\end{quote}

Reply: 
We included the G mag and colours in Table 1.

\begin{quote}
    - C5. Table 1 has incorrect observation dates , an HJD of 58428 corresponds to -4553!

\end{quote}

Reply: 
Thank you for pointing out this. We are reporting in Table 1 the reduced Heliocentric Julian Day, RHJD = HJD - 2400000. We have changed the heading of this column in RHJD to avoid confusion. 

\begin{quote}
    - C6. Section 2, Par 4: Insert references for text: “..surface He abundance...affected by microscopic diffusion” and following text. More detail is needed about the calculations shown in Fig. 2.
\end{quote}

Reply: We have added more descriptions about the isochrone we use in fig. 2, and referred to the corresponding stellar model papers for more details on the diffusion process.

\begin{quote}
    - C7. Fig 1 caption: Identify the color system.

\end{quote}

Reply: The colour system in Fig. 1 is Gaia DR2 photometry. We added the corresponding description to the caption.

\begin{quote}
    - C8. Fig. 5: Define “Kiel diagram”

\end{quote}

Reply: 
We add the definition, 'i.e. Teff - logg', for clarity.

\begin{quote}
    - C9. Section 4.1: Introduction of the “peak wavelength” is confusing. Peak means maximum... .. isn’t the wavelength at the minimum value of the profile meant here and subsequently?
\end{quote}

Reply: 
We replaced the "peak wavelength" with "line center wavelength", and also use the notation $\lambda_\mathrm{centre}$ instead of $\lambda_\mathrm{peak}$. The relevant words in section 4.1 are also modified.   

\begin{quote}
    - C10. Fig. 9: R in figure is not defined.
\end{quote}

Reply: We defined the Pearson correlation coefficient in Fig. 9. To better distinguish the correlation coefficient and resolution, we also use 'r' instead of 'R' in the figure.

We also take the chance to modify the other contents in the manuscript, including typos, and more complete references. 

\end{document}
